# Supplementary material for: One-step Diffusion with Distribution Matching Distillation
Source: arXiv:2311.18828 source file (2024-10-04)

create an image that depicts a majestic kingdom with towering castles, lush gardens, and vibrant colors. show the bustling streets filled with lively townsfolk and capture the enchanting atmosphere of the realm.”

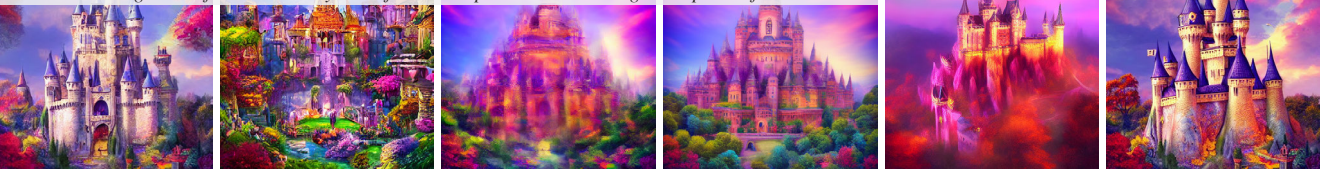

“fluffy little ball of fur with cute eyes holding a tiny spear in a fantasy forest, being chased by a giant hand”

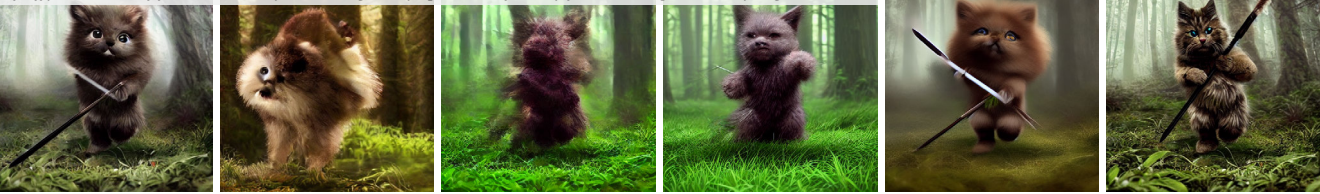

“an underwater photo portrait of a beautiful fluffy white cat, hair floating. In a dynamic swimming pose. The sun rays filters through the water. High-angle shot. Shot on Fujifilm X”

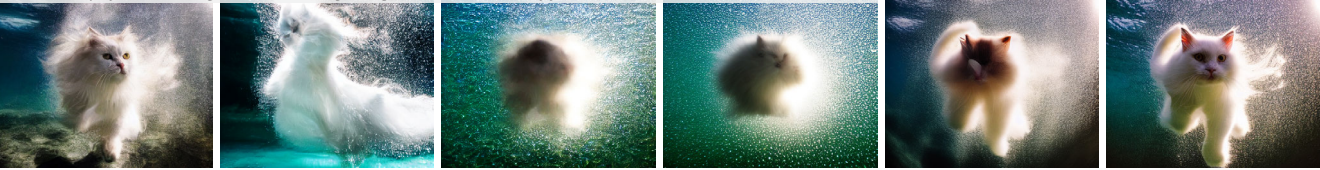

“transparent vacation pod at dramatic scottish lochside, concept prototype, ultra clear plastic material, editorial style photograph”

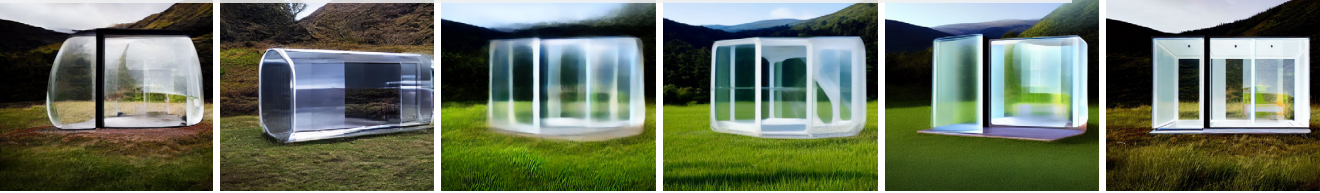

“3D animation cinematic style young caveman kid, in its natural environment”

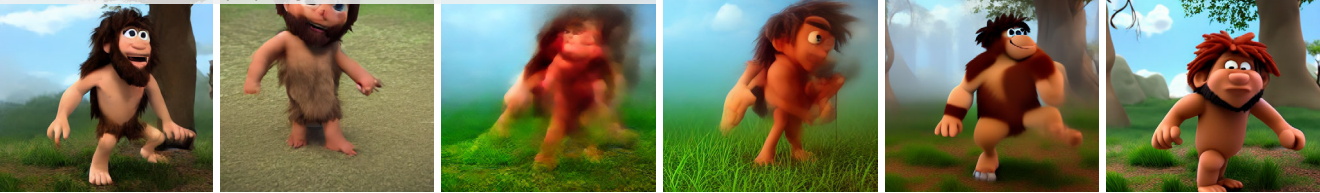

“robot with human body form, robot pieces, knolling, top of view, ultra realistic”

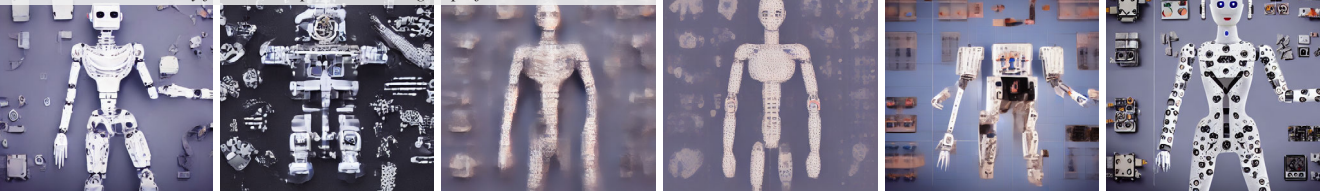

DMD (ours, 1 step)  
90ms

InstaFlow (1 step)  
90ms

LCM (1 step)  
90ms

LCM (2 steps)  
120ms

DPM++ (4 steps)  
260ms

SD (50 steps)  
2590ms

*ects a majestic kingdom with  
lled with lively townsfolk and*

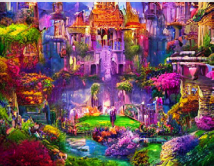

Supplement: Supplementary file 1 [file more_results.pdf]
